# Supplementary material for: Robust Analytics for Video-Based Gait Biometrics
Source: arXiv:2111.06670 source file (2021-11-12)
Supplement: Supplementary file 1 [file appendix.tex]

\appendix
\addcontentsline{toc}{chapter}{APPENDIX}
\chapter{Topic 1}
\section{Section 1}
\section{Section 2}
\chapter{Topic2}
\label{sec:topic2}
\newpage
\chapter{Topic3}
\label{chap:topic3}
